# Supplementary material for: DiMeR: Disentangled Mesh Reconstruction Model
Source: arXiv:2504.17670 source file (2025-05-26)
Supplement: Supplementary file 1 [file appendix.tex]

\section{Additional Results of Ablation Studies}
To validate the inefficiency of deformation and weight networks in FlexiCubes, we additionally conduct the experiments based on the official pre-trained weights of PRM.
As shown in Tab.~\ref{tab: deformation based on PRM}, removing these two networks doesn't damage the performance.

\begin{table}[h]
\centering
\tabcolsep=0.8cm
\resizebox{0.6\linewidth}{!}{
\begin{tabular}{l|cc}
\toprule
Method      & CD & F1  \\ \midrule
w/ & 0.041   &  0.977   \\
w/o & 0.041   & 0.977 \\ 
\bottomrule
\end{tabular}}
\caption{The ablation studies of the effectiveness of Deformation and Weight MLP based on PRM. GPU Mem is training occupancy.}
\label{tab: deformation based on PRM}
\end{table}

\section{More Visual Results}

\begin{figure}[h]
    \centering
    \includegraphics[width=1\linewidth]{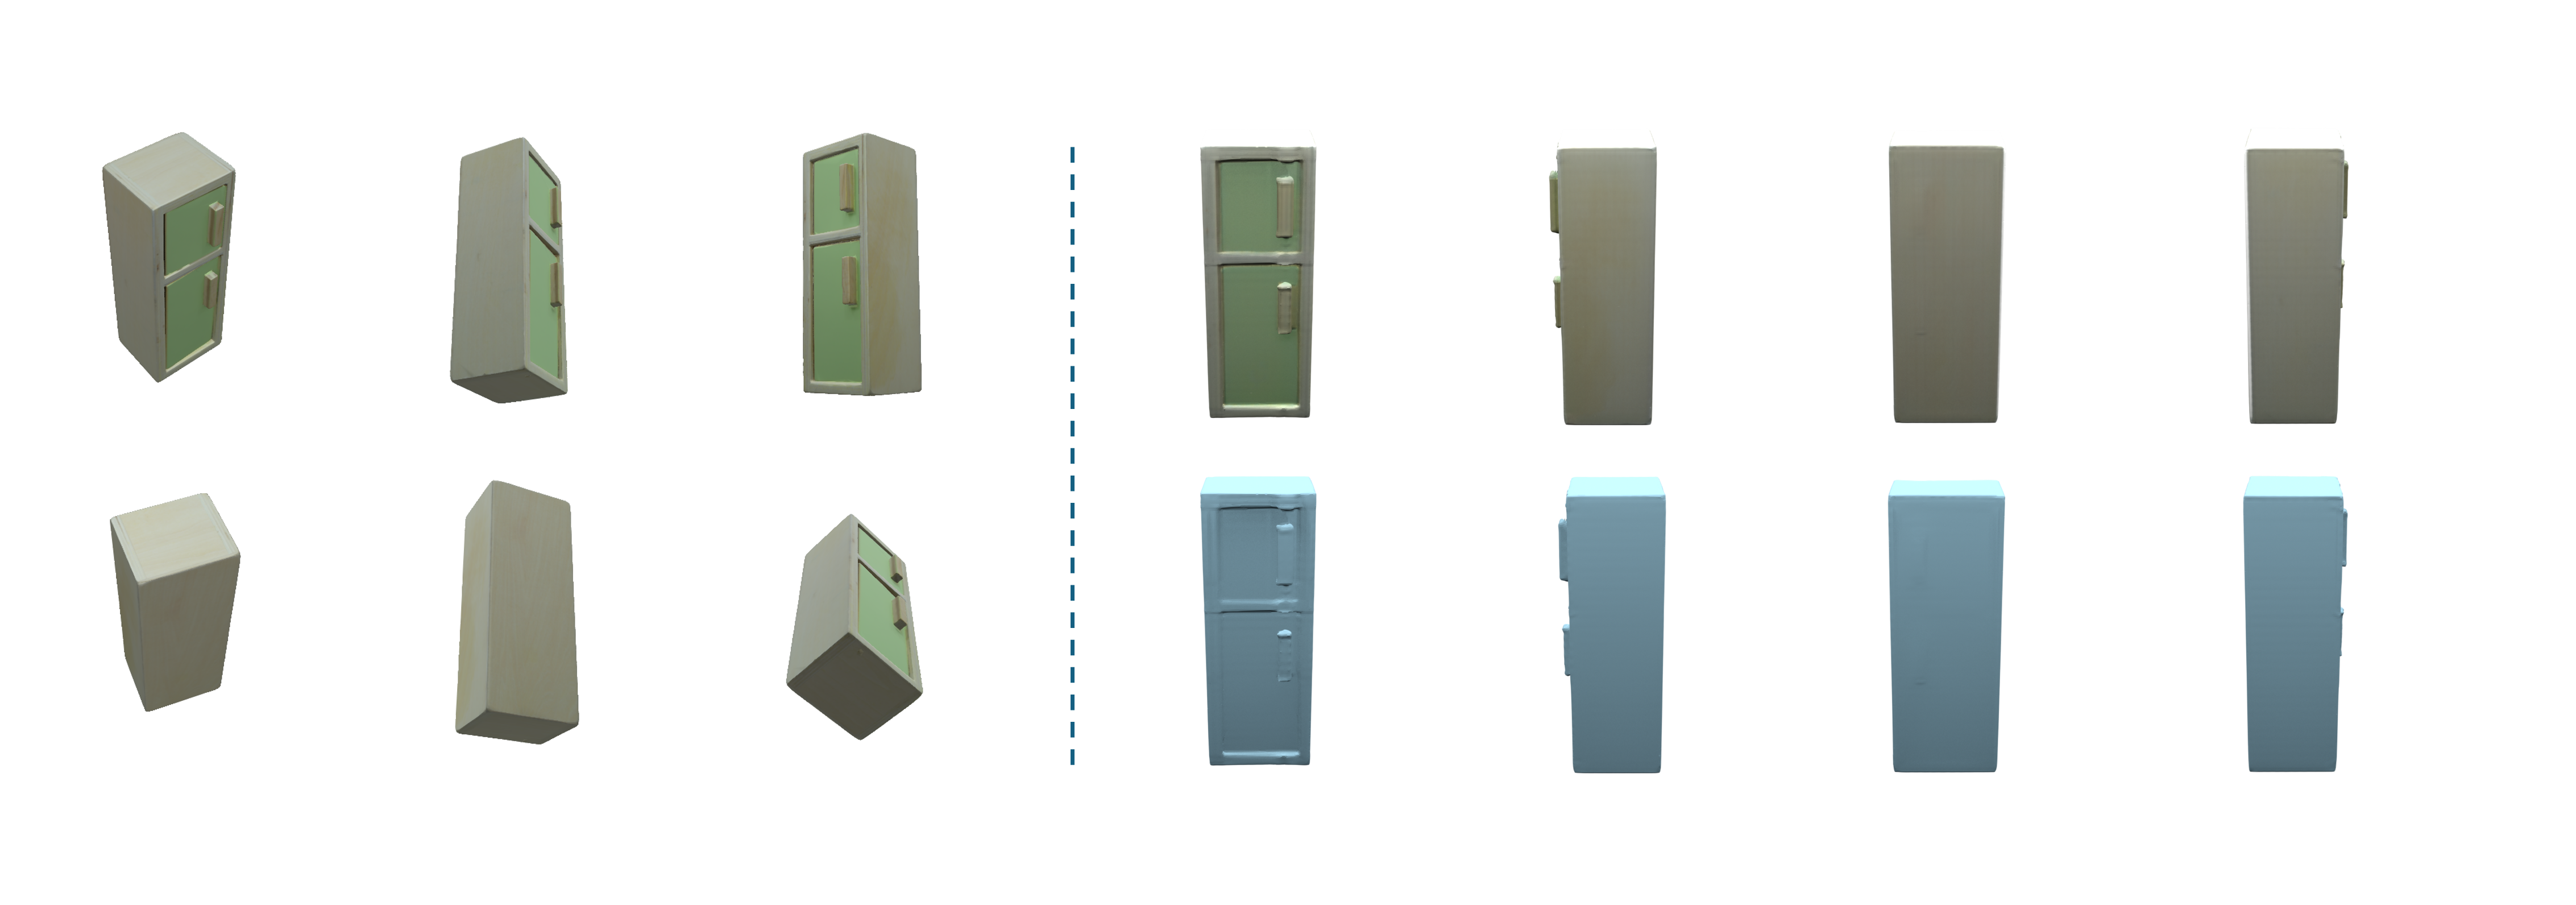}
\end{figure}

\begin{figure}[h]
    \centering
    \includegraphics[width=1\linewidth]{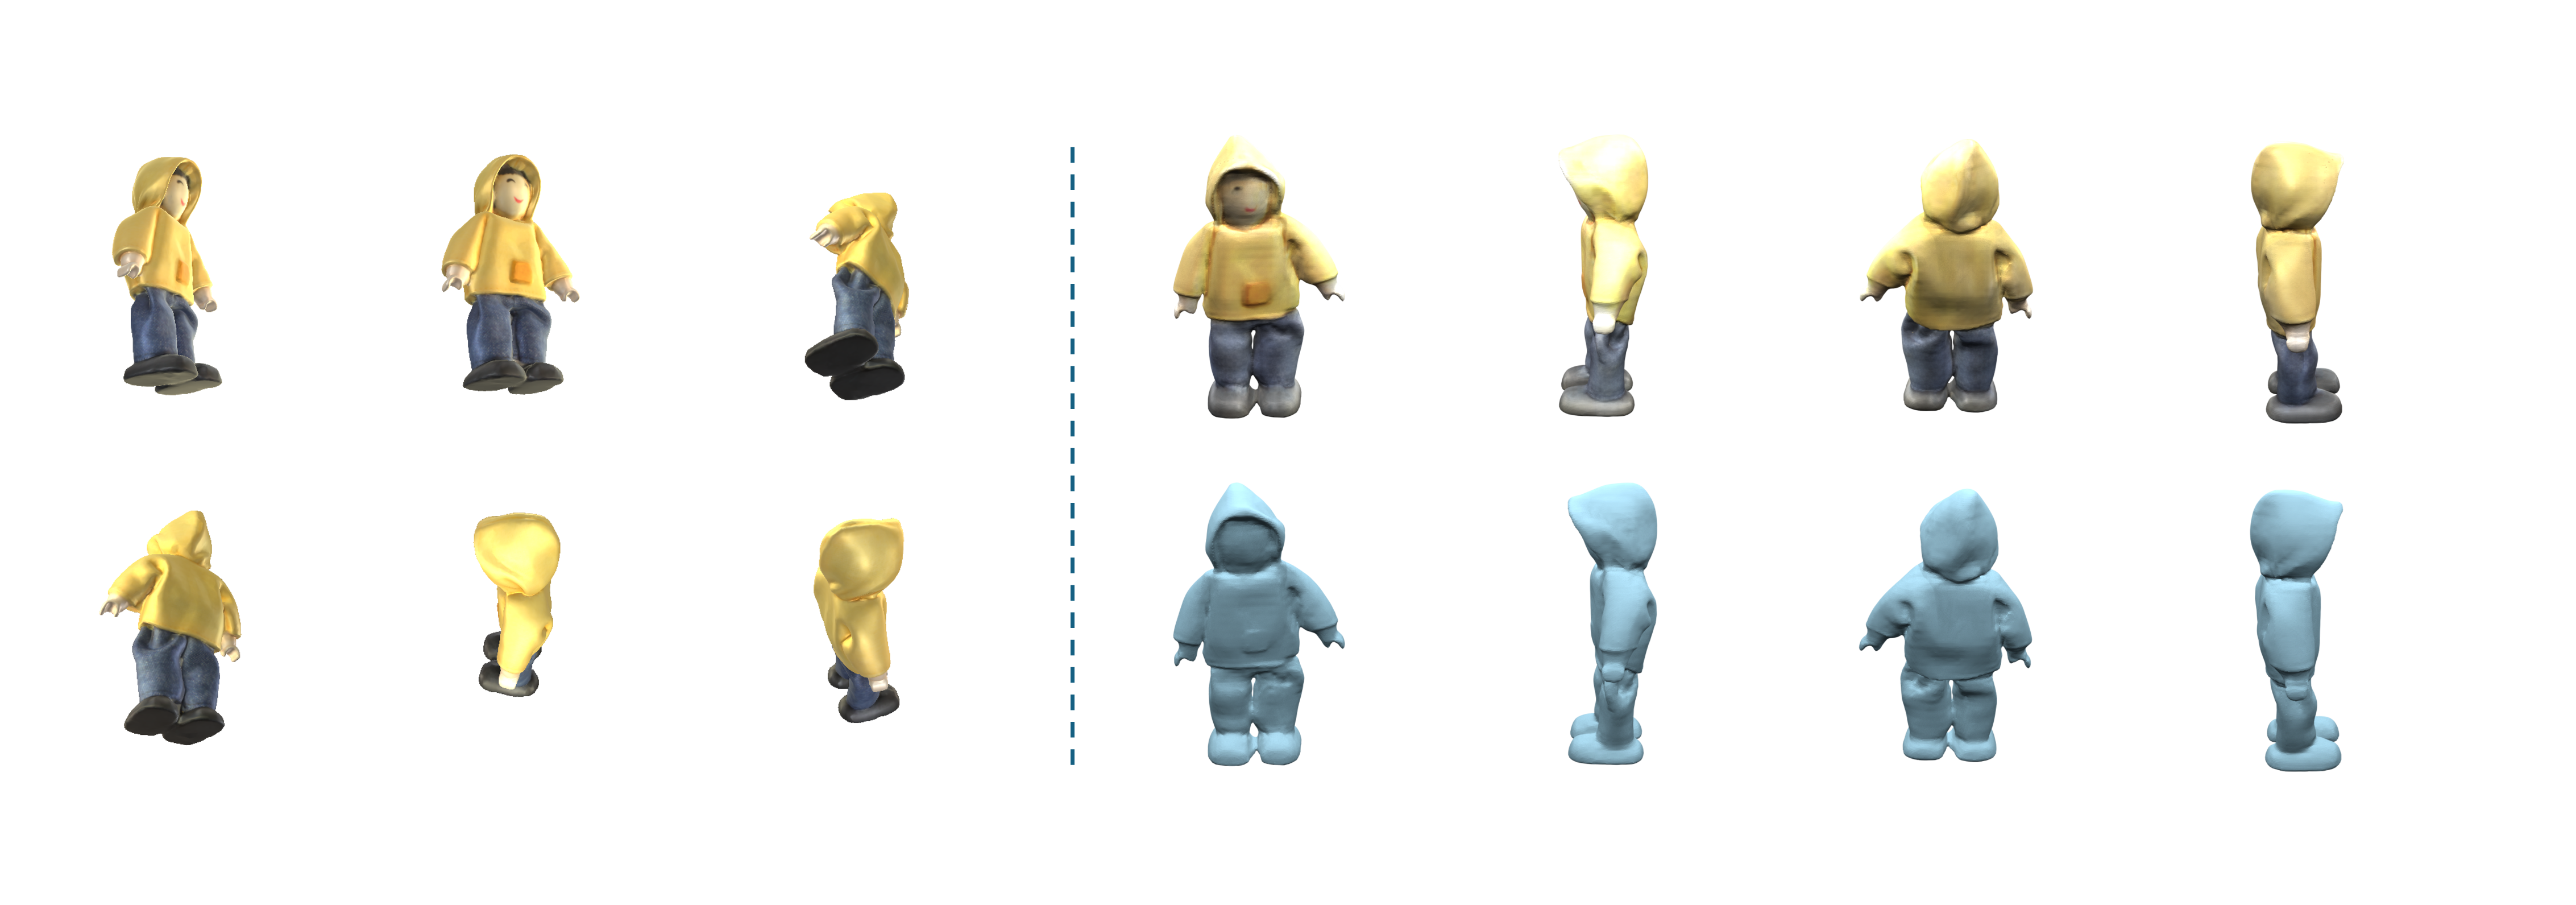}
\end{figure}

\begin{figure}[h]
    \centering
    \includegraphics[width=1\linewidth]{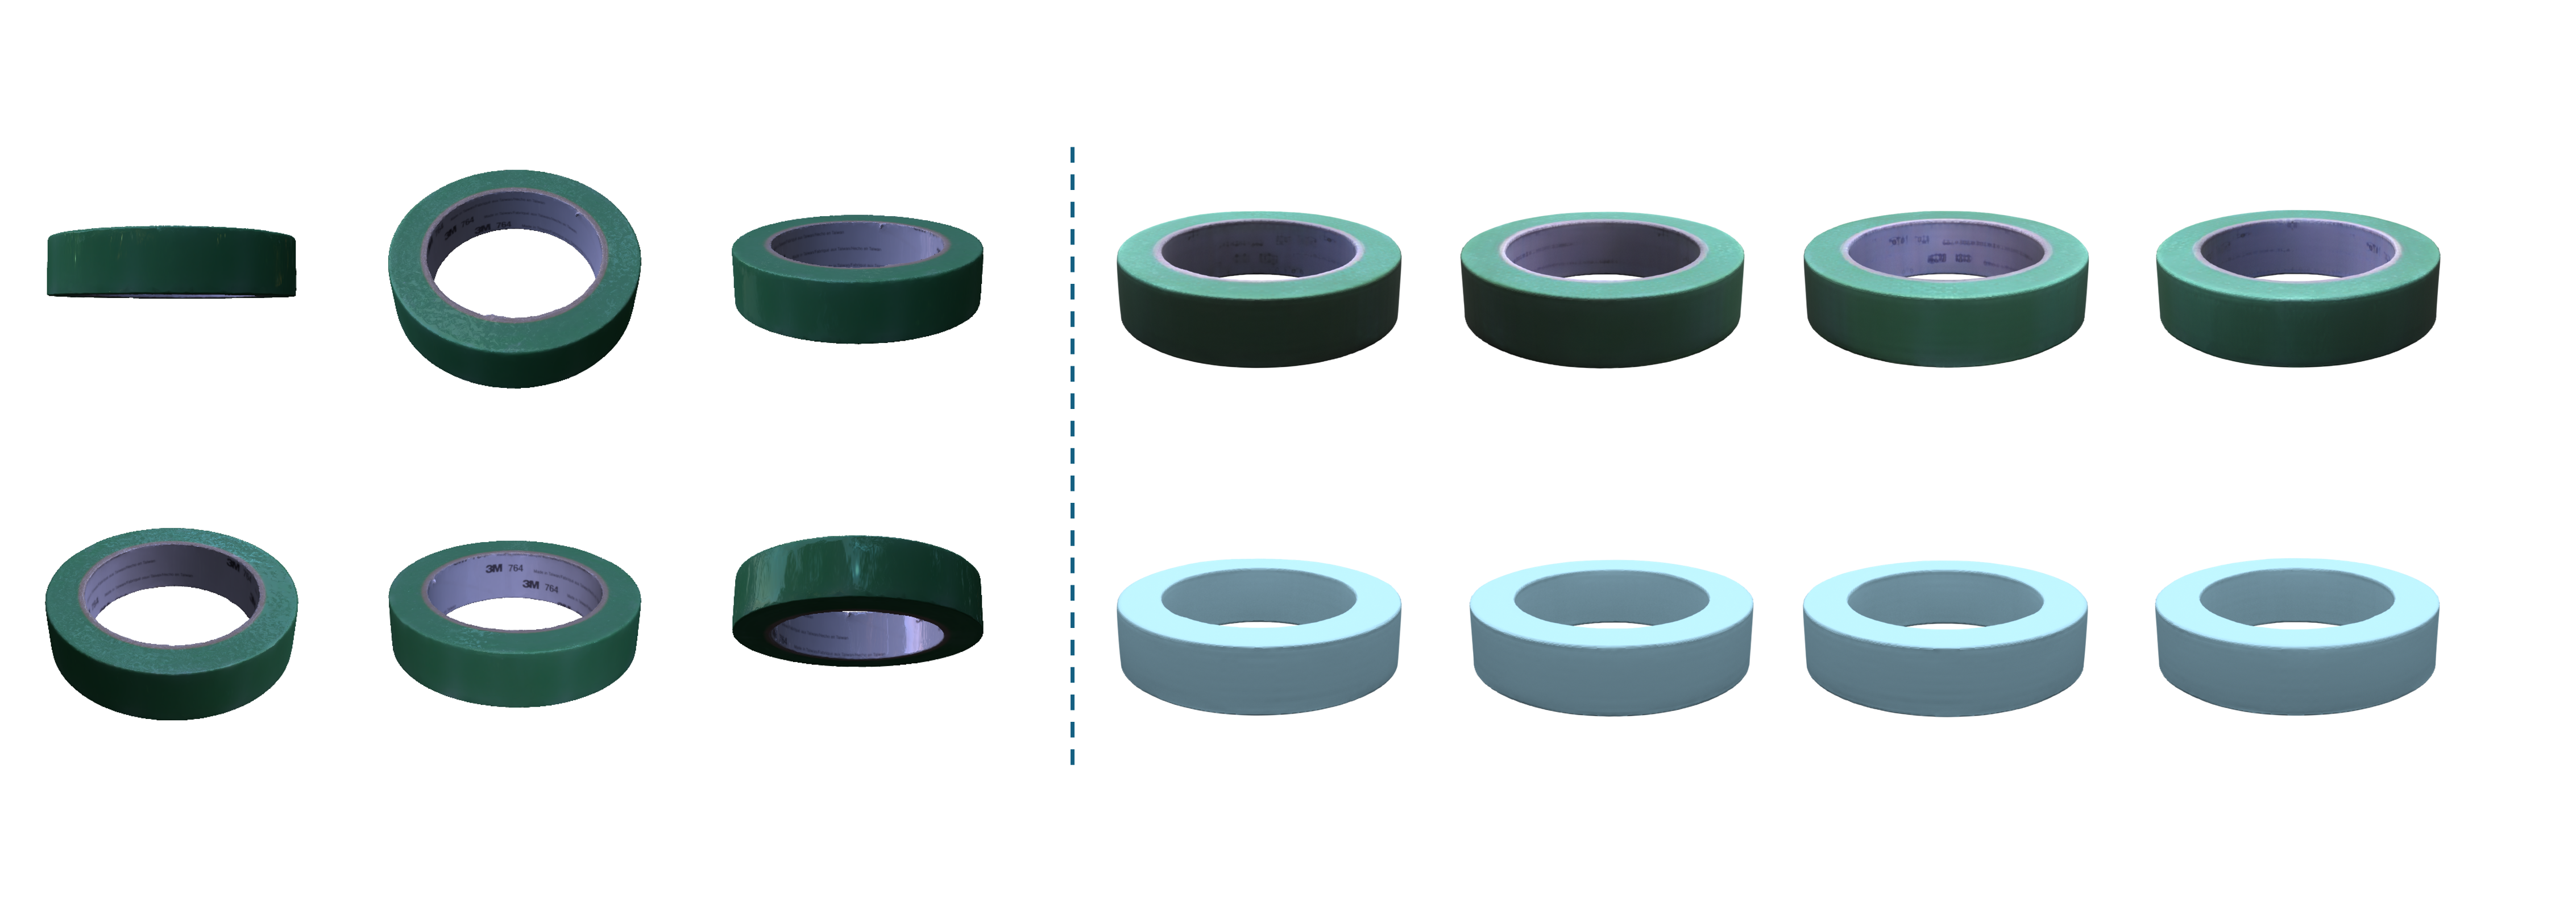}
\end{figure}

\begin{figure}[h]
    \centering
    \includegraphics[width=1\linewidth]{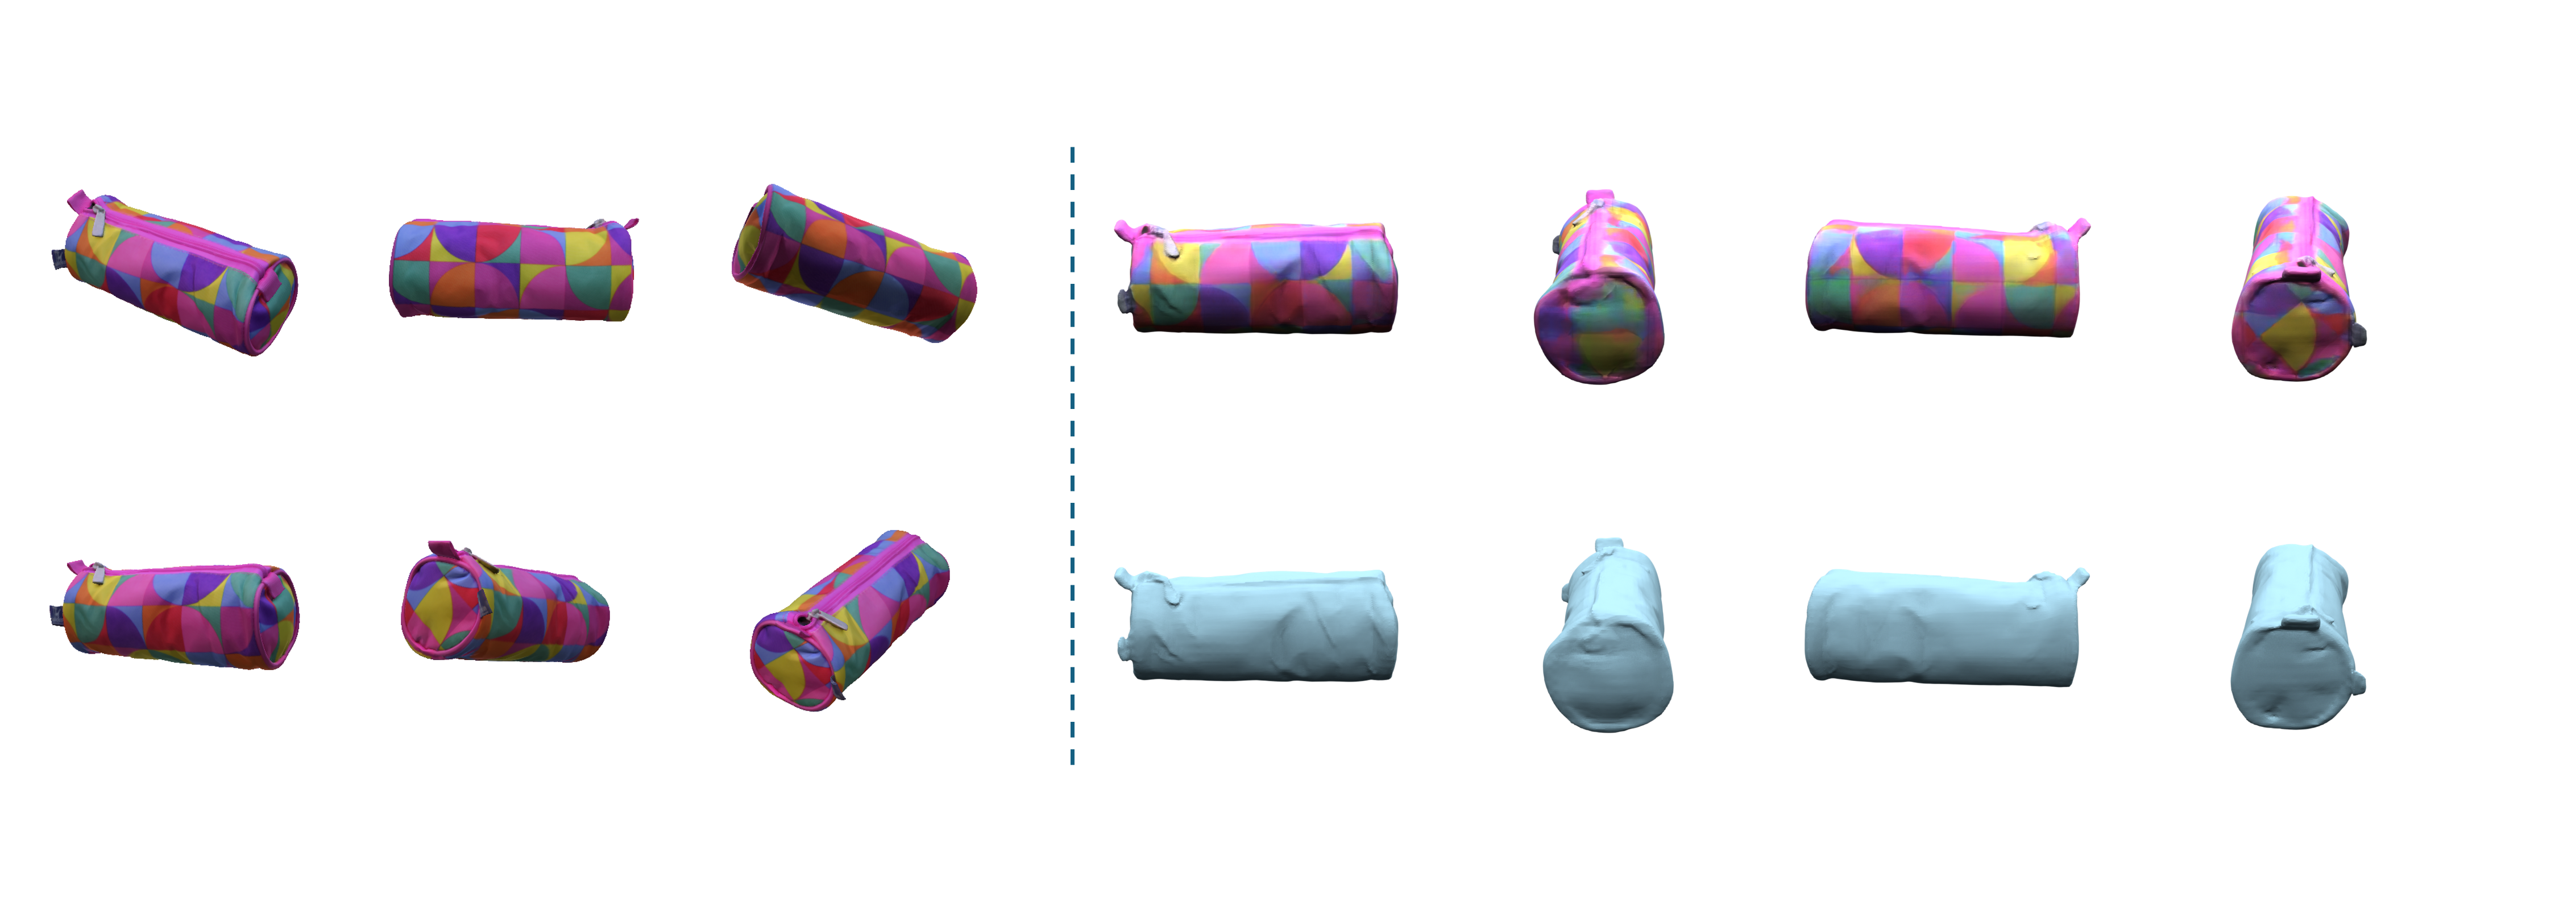}
\end{figure}

\begin{figure}[h]
    \centering
    \includegraphics[width=1\linewidth]{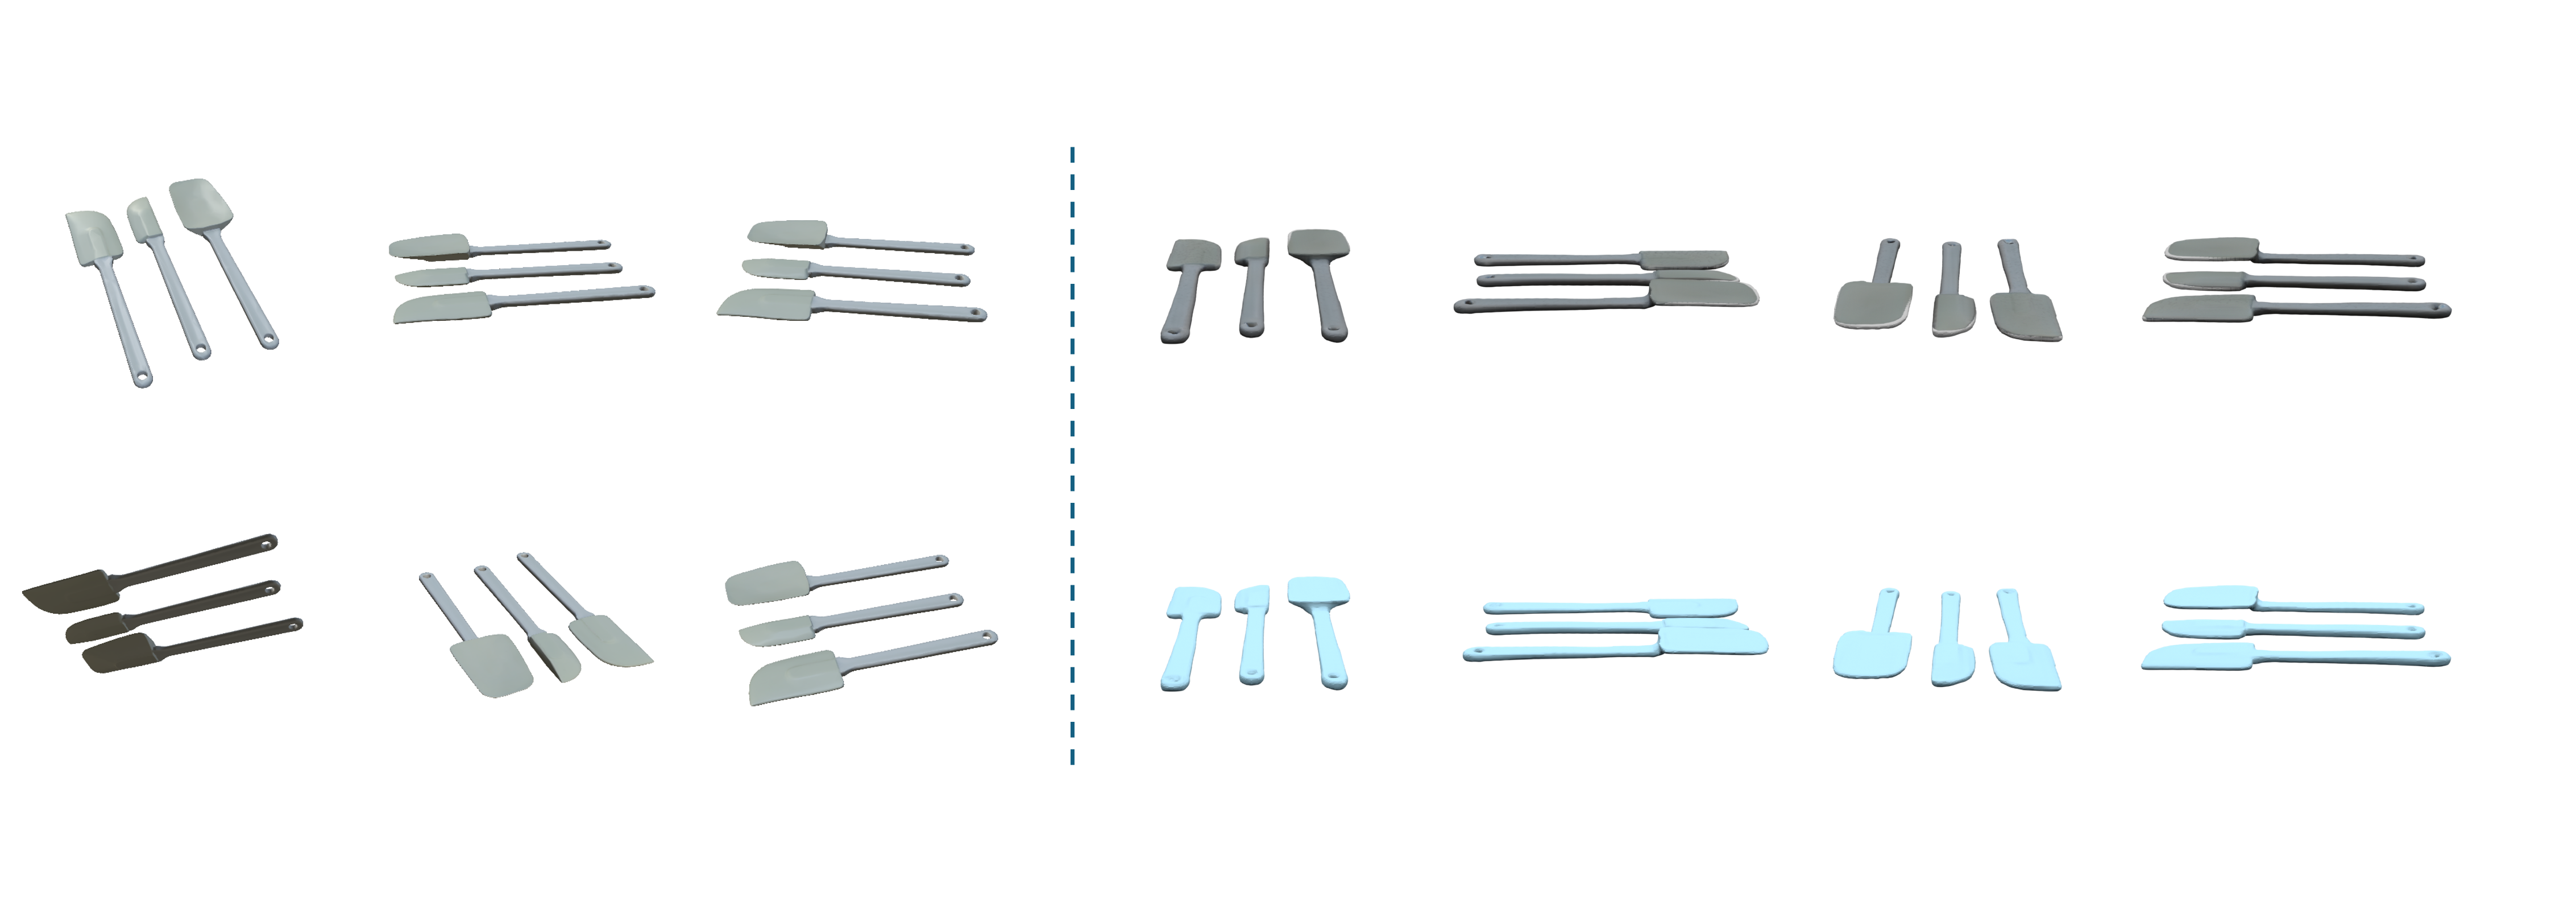}
\end{figure}

\begin{figure}[h]
    \centering
    \includegraphics[width=1\linewidth]{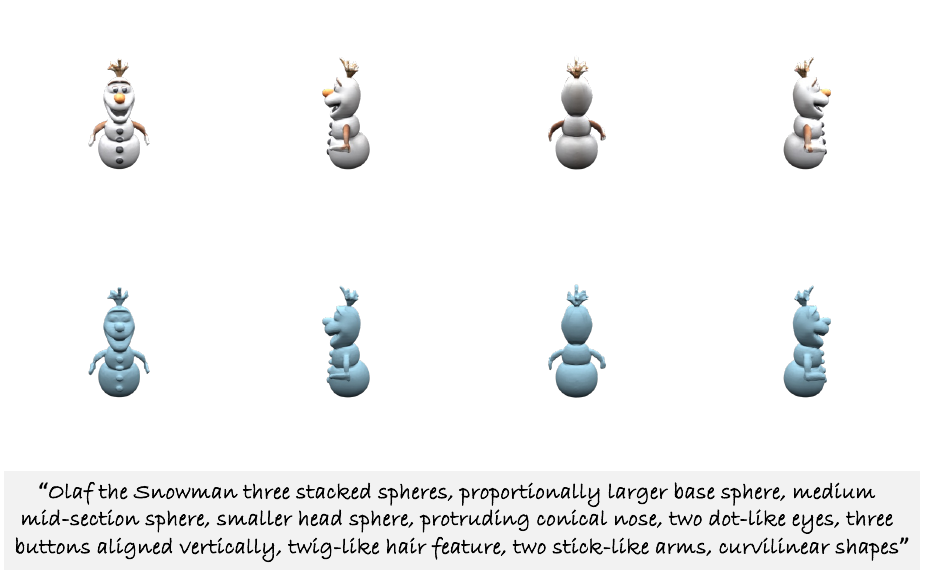}
\end{figure}

\begin{figure}[h]
    \centering
    \includegraphics[width=1\linewidth]{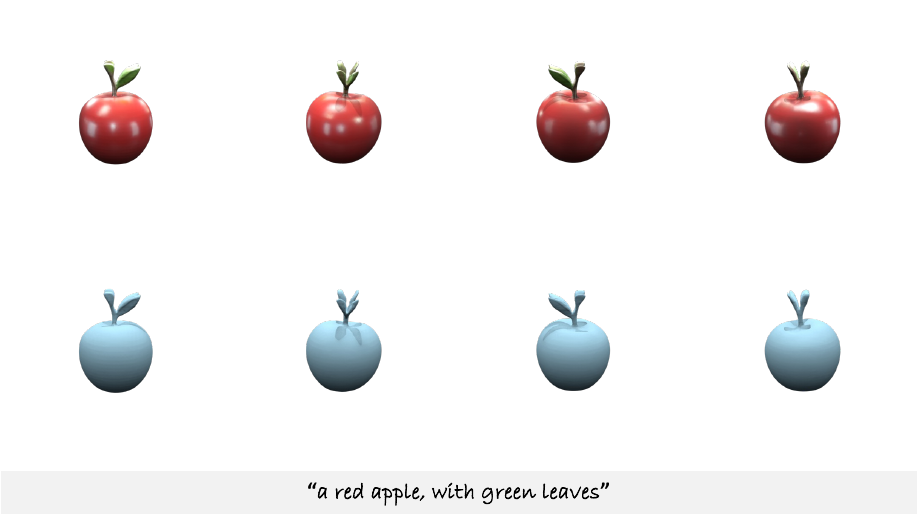}
\end{figure}

\begin{figure}[h]
    \centering
    \includegraphics[width=1\linewidth]{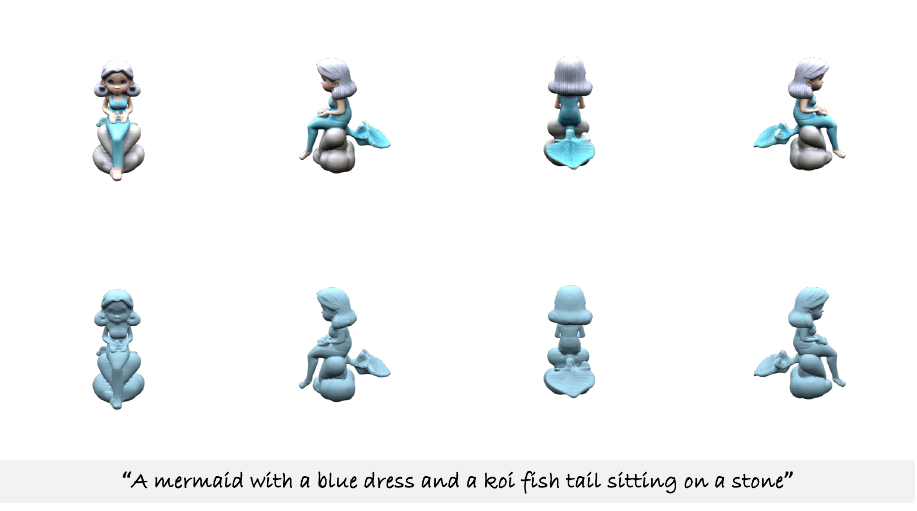}
\end{figure}

\begin{figure}[h]
    \centering
    \includegraphics[width=1\linewidth]{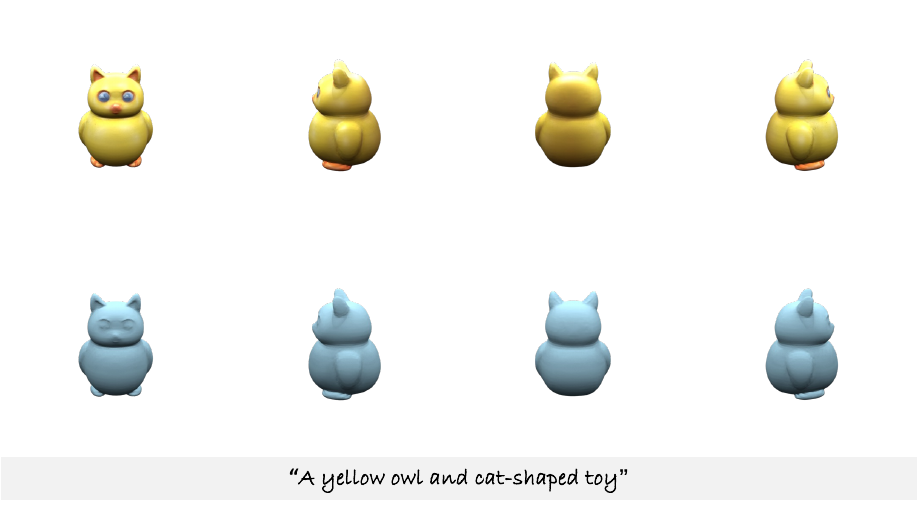}
\end{figure}

\begin{figure}[h]
    \centering
    \includegraphics[width=1\linewidth]{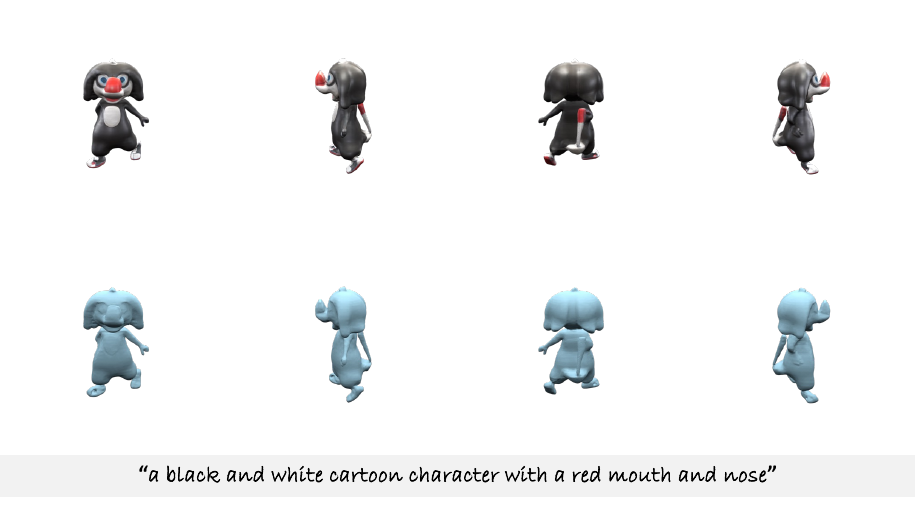}
\end{figure}

\begin{figure}[h]
    \centering
    \includegraphics[width=1\linewidth]{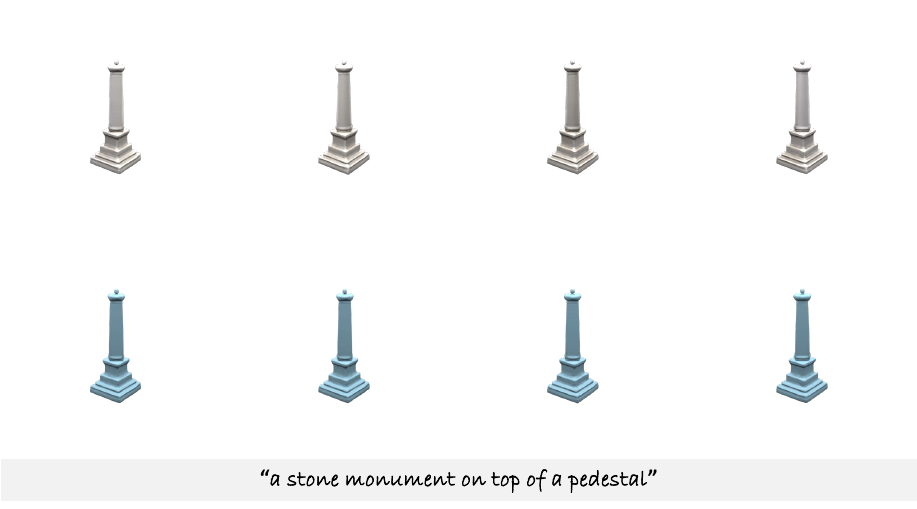}
\end{figure}

\begin{figure}[h]
    \centering
    \includegraphics[width=1\linewidth]{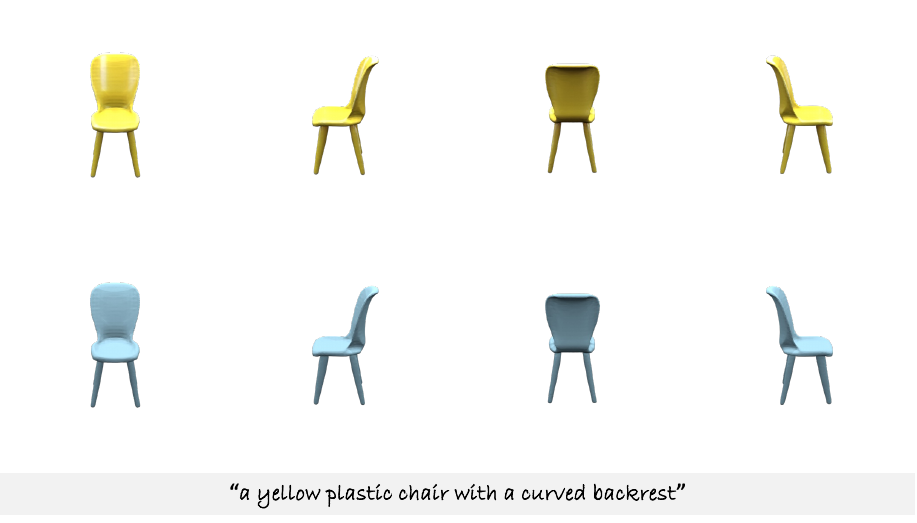}
\end{figure}

\begin{figure}[h]
    \centering
    \includegraphics[width=1\linewidth]{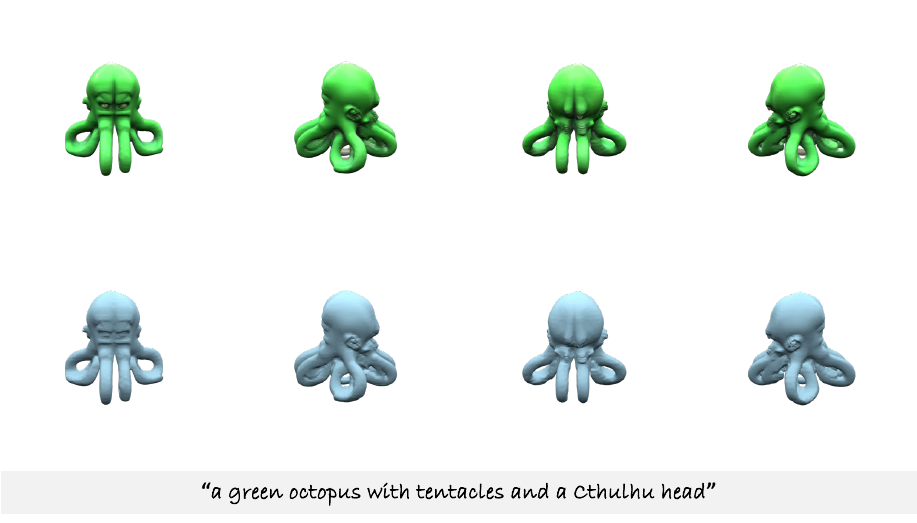}
\end{figure}

\begin{figure}[h]
    \centering
    \includegraphics[width=1\linewidth]{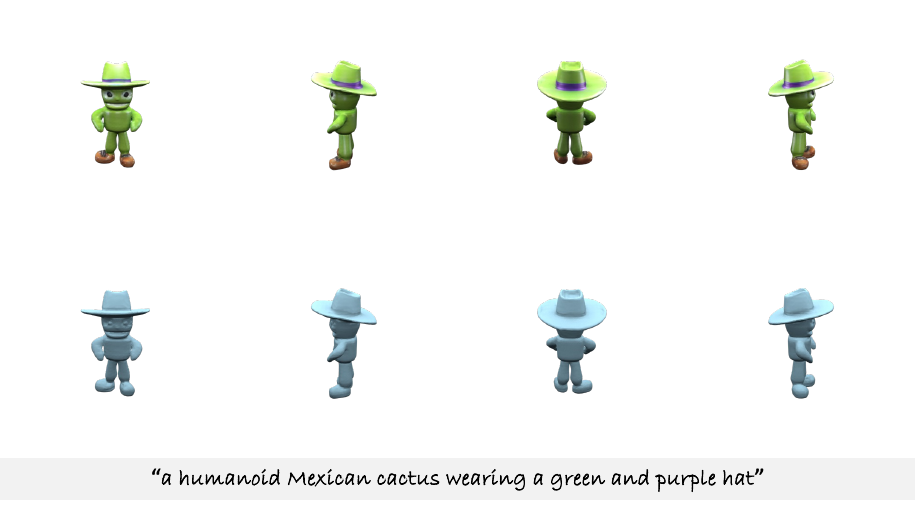}
\end{figure}

% \begin{figure}[h]
%     \centering
%     \includegraphics[width=1\linewidth]{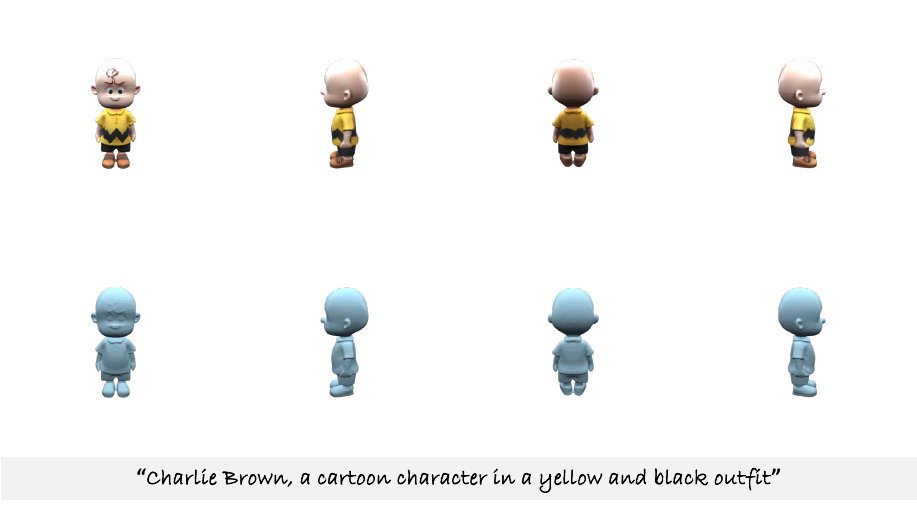}
% \end{figure}

\begin{figure}[h]
    \centering
    \includegraphics[width=1\linewidth]{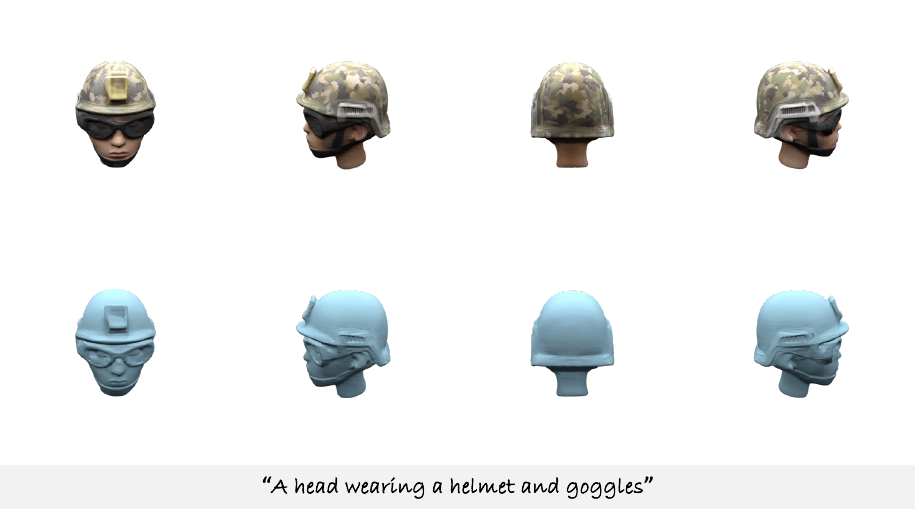}
\end{figure}

% \begin{figure}[h]
%     \centering
%     \includegraphics[width=1\linewidth]{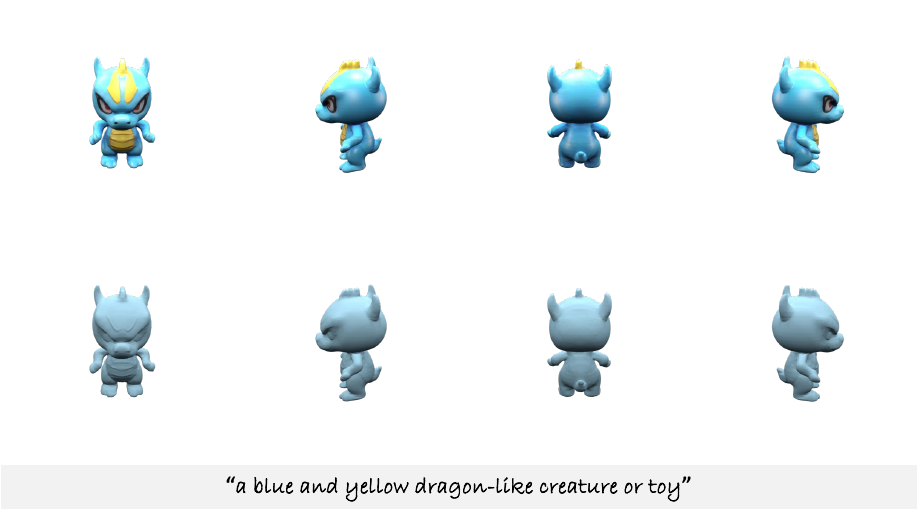}
% \end{figure}

\begin{figure}[h]
    \centering
    \includegraphics[width=1\linewidth]{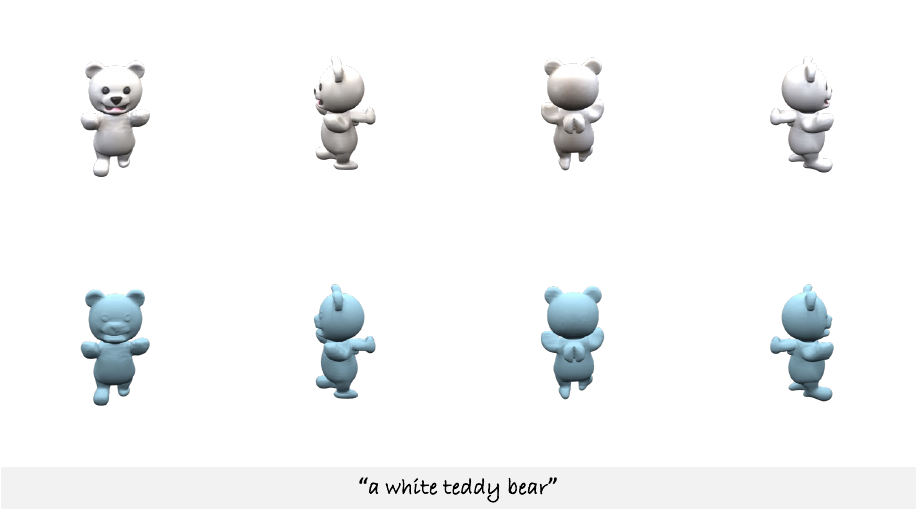}
\end{figure}

\begin{figure}[h]
    \centering
    \includegraphics[width=1\linewidth]{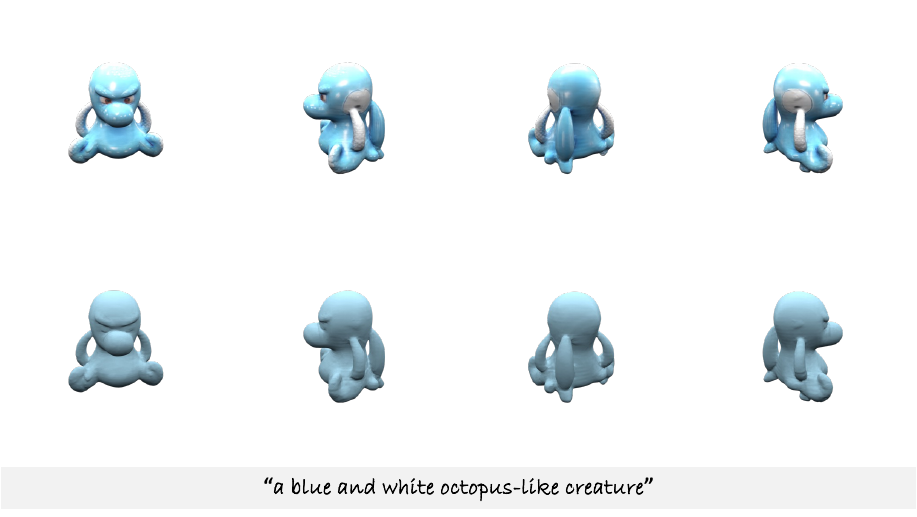}
\end{figure}

\begin{figure}[h]
    \centering
    \includegraphics[width=1\linewidth]{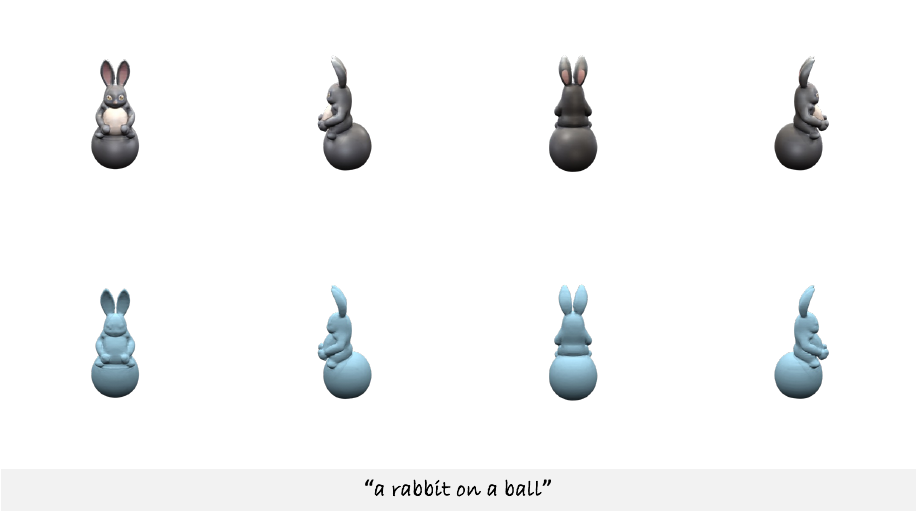}
\end{figure}

\begin{figure}[h]
    \centering
    \includegraphics[width=1\linewidth]{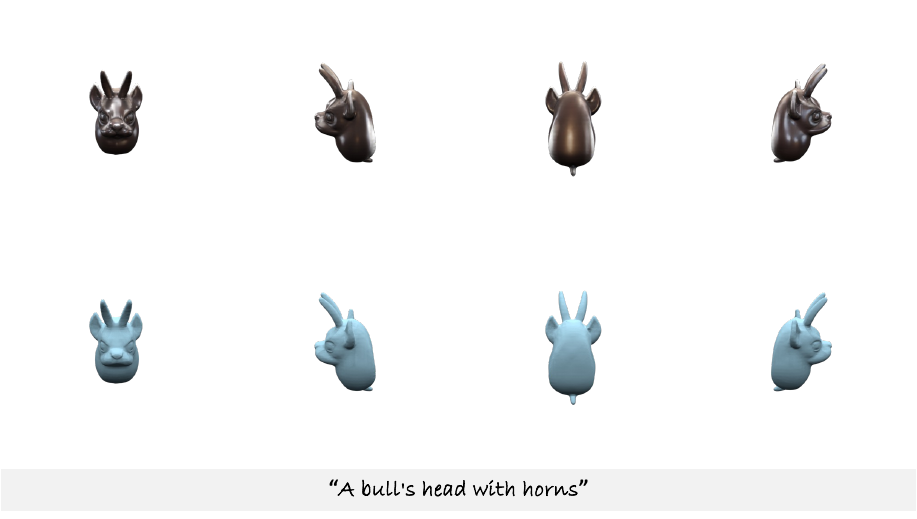}
\end{figure}

\begin{figure}[h]
    \centering
    \includegraphics[width=1\linewidth]{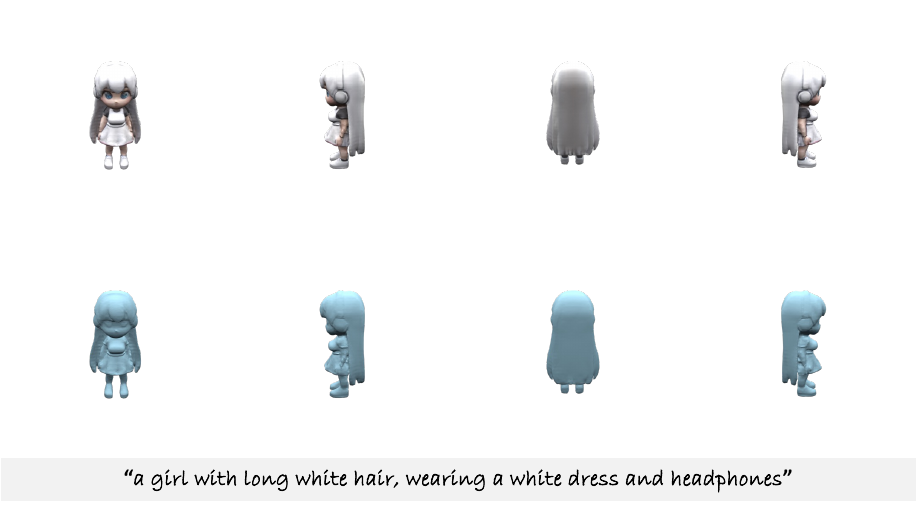}
\end{figure}

\begin{figure}[h]
    \centering
    \includegraphics[width=1\linewidth]{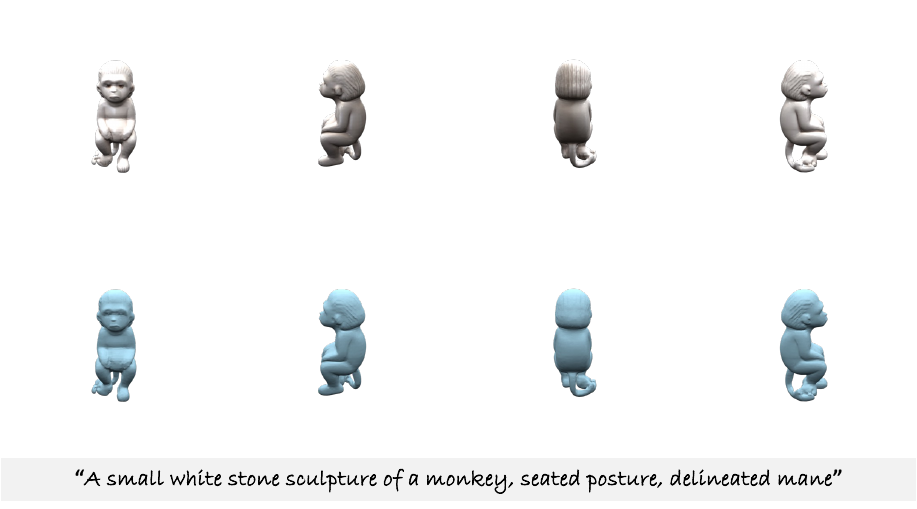}
\end{figure}

\begin{figure}[h]
    \centering
    \includegraphics[width=1\linewidth]{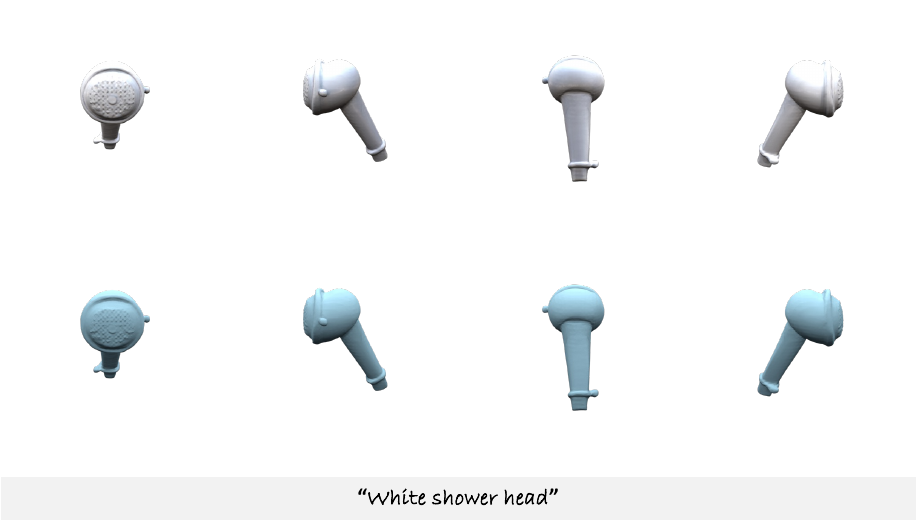}
\end{figure}

\begin{figure}[h]
    \centering
    \includegraphics[width=1\linewidth]{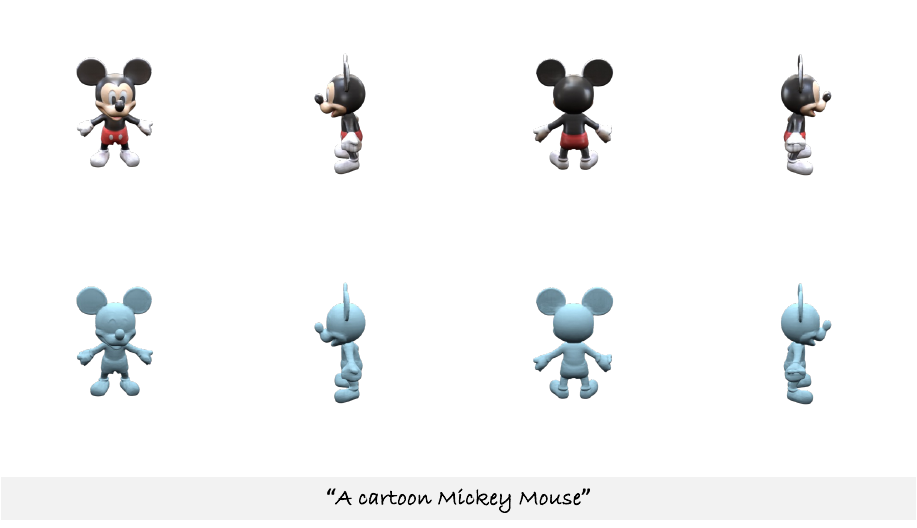}
\end{figure}

\clearpage
